# Supplementary material for: The Moral Mind(s) of Large Language Models
Source: arXiv:2412.04476 source file (2025-04-25)
Supplement: Supplementary file 1 [file supplementary_information.tex]

\clearpage

 {\LARGE \  \noindent \textbf{Supplementary Information} }
 
\section{Recovering Preferences}\label{section: preferences main}

This section shows that when a model is rational, i.e., when GARP$_\mathbf{e}$ is satisfied at the highest level, $\mathbf{e=1}$, then all observed answers are maximizing a utility function. The result below draws on \cite{seror2024pricedsurveymethodologytheory}. As I will show next, the utility functions rationalizing PSM answers is singled-peaked. I define a single-peaked function as follows:
\begin{definition}\label{def: single peaked}
A function $f:X\rightarrow \mathbb{R}$ is single-peaked if
\begin{itemize}
    \item There exists a point $\mathbf{y^*}\in \mathbb{R}^S$ such that $f(\mathbf{y})\leq f(\mathbf{y^*})$ for any $\mathbf{y}\in X$.
    \item For any $\mathbf{x}, \mathbf{y} \in X$ such that $\mathbf{x}_c\leq \mathbf{y_c}\leq \mathbf{y^*_c}$ for $\mathbf{c} \in C(\mathbf{X})$, $f(\mathbf{x})\leq f(\mathbf{y})\leq f(\mathbf{y^*})$. 
\end{itemize}
\end{definition}
The second condition means that if it is possible to rank $x,y,y^*$ as $\mathbf{x_c\leq y_c\leq y^*_c}$ in a given coordinate system $c$, then $f(\mathbf{x})\leq f(\mathbf{y})$ as $\mathbf{x}$ is further away than $\mathbf{y}$ in the coordinate system $\mathbf{c}$. I define single-peaked preferences as follows:
\begin{definition}\label{Def: single peaked pref}
   A preference relation $\succcurlyeq$ is  single-peaked with respect to the order pair $(\geq, >)$ if there exists a unique $\mathbf{y}^*\in \mathbb{R}^S$ such that for any $\mathbf{x,y}\in X$, $\mathbf{x_c\leq y_c\leq y_c^*}$ for some $\mathbf{c}\in C(X)$, iif $y \succcurlyeq x$ and $\mathbf{x_c< y_c\leq y_c^*}$ iff $y \succ x$, with $\succ$ the strict part of $\succcurlyeq$. 
\end{definition}
Before turning to the Theorem, one last assumption is necessary:
\begin{assumption}
     The vertex $\mathbf{c=o^k}$ associated to round $k\in \mathcal{R}$ is the unique vertex that satisfies the condition $\mathbf{c}\leq \mathbf{q}< \mathbf{q^0_c}$ for some $\mathbf{q}\in \mathcal{B}^k$.
\end{assumption}

This assumption is made to ensure that the pre-order of the set \( X \), in round $k$, is monotonic in the coordinate system originating in \(\mathbf{o^k}\). Specifically, the assumption implies that in coordinate system originating in \(\mathbf{o^k}\), any model face a trade off between increasing the answer to one question with increasing the answer to the other questions.\footnote{Condition $\mathbf{q}< \mathbf{q^0_c}$ implies that $\mathbf{p^k.q}< \mathbf{p^k.q^0_c}$ for any $\mathbf{q}\in \mathcal{A}^r$.} Concretely, consider an example where the ideal answer is $\mathbf{q^*}=(2,2,2,2,2)$. Answer $\mathbf{q^1}=(4,4,3,2,4)$ should always be preferred to answer $\mathbf{q^2}=(5,4,5,5,5)$, because  $\mathbf{q^1}$ is closer to $(2,2,2,2,2)$ than $\mathbf{q^2}$. This can be seen by changing the coordinate system. In the coordinate system originating in $\mathbf{c}=(5,5,5,5,5)$, $\mathbf{q^1_c}=(1,1,2,3,1)$,  $\mathbf{q^2_c}=(0,1,0,0,0)$, and $\mathbf{q^*_c}=(3,3,3,3,3)$.

A utility function $u: X\rightarrow \mathbb{R}$ weakly rationalizes the data if for all $k$ and $\mathbf{y}\in X$,  $\mathbf{p^k.q^k_{o^k}\geq p^k. y_{o^k}}$ implies that $u(\mathbf{q^k})\geq u(\mathbf{y})$. Similarly, a preference relation $\succcurlyeq$ weakly rationalizes the data iif the revealed preference pair $(R^0, P^0)$ satisfies $R^0\subset \succcurlyeq$. The following result is established by \cite{seror2024pricedsurveymethodologytheory}:
\begin{theorem}\label{theorem: halevy}
The following conditions are equivalent:
\begin{enumerate}
\item $D$ has a weak single-peaked rationalization. 
    \item The data satisfy $\text{GARP}$.

    \item There are strictly positive real numbers $U^k$ and $\lambda^k$, for each $k$ such that
    \begin{equation}\label{eq: afriat}
        U^k\leq U^l+\lambda^l \mathbf{p^l} (\mathbf{q^k_{o(l)}} - \mathbf{q^l_{o(l)}})
    \end{equation}
    for each pair of observations $(\mathbf{q^k}, \mathbf{\mathcal{B}^k}), (\mathbf{q^l}, \mathbf{\mathcal{B}^l})$ in $D$.
        \item $D$ has a single-peaked, continuous, concave utility function that rationalizes the data.
\end{enumerate}
\end{theorem}

There exists a utility function that exactly rationalizes all observed answers as utility-maximizing when GARP is satisfied. If $\mathbf{o^k=0}$ for all rounds, then Theorem \ref{theorem: halevy} is the standard version of \citeauthor{afriat1967}'s theorem. However, unlike the standard theorem, according to Theorem  \ref{theorem: halevy}, the rationalizing utility function is single-peaked rather than monotonic. This distinction offers several advantages, which will be further discussed in the application section. Briefly, single-peakedness allows us to obtain an ordinal measure of preferences that avoids the interpretational issues of traditional scale-based measures. Additionally, the peak of the utility function is defined in a continuous space, making it robust to common survey limitations such as scale bounds and order effects. Finally, using a single-peaked utility function within the PSM framework enables us to capture nuanced aspects of preferences, such as the relative importance that models assign to different survey items, thereby offering a more structured and adaptable approach to understanding moral preferences.
